# Supplementary material for: Unified description of the $Qs \bar q \bar q$ molecular bound states, molecular resonances and compact tetraquark states in the quark potential model
Source: arXiv:2310.14597 source file (2024-01-14)
Supplement: Supplementary file 1 [file supplemental.tex]

\setcounter{equation}{0}
\setcounter{figure}
{0}
\setcounter{table}{0}

This supplemental material provides additional details on...

\maketitle

\section{xxx}
